# Supplementary material for: The importance of better models in stochastic optimization
Source: arXiv:1903.08619 source file (2019-03-20)
Supplement: Supplementary file 1 [file appendix-stab.tex]

% -*- Mode: latex -*- %

\section{Proofs of stability results}

\subsection{Proof of Lemma~\ref{lemma:stab-weakly-conv_1}}
\textcolor{red}{which version of SPPM should we use here? I guess the one with $f_{x_k}(x) = f(x) + \frac 1 2 \rho \ltwo{x-x_k}^2 $.}

\subsection{Proof of Lemma~\ref{lemma:stab-weakly-conv_2}}

\subsection{Proof of Theorem~\ref{theorem:stab_prox_linear_1}}

\subsection{Proof of Theorem~\ref{theorem:stab_prox_linear_2}}
